# Supplementary material for: Follow Me at the Edge: Mobility-Aware Dynamic Service Placement for Mobile Edge Computing
Source: arXiv:1809.05239 source file (2018-09-14)
Supplement: Supplementary file 3 [file appendix3.tex]

\appendices

\section{\textbf{Proof of Lemma~\ref{lemma-drift}}}
\label{sec:lem-drift-appendix}

\begin{IEEEproof}
For $\Delta(\Theta(t))$, obviously, we can square equation (\ref{expressionOfQueue}) and use the fact that $ (max[Q-b+A,0])^2  \le Q^2 +A^2 +b^2 +2Q(A-b)$ for any $Q, b, A \ge 0 $ to obtain the following inequality:
\begin{small}
\begin{equation}
\begin{aligned}
    L(\Theta(t + 1)) - L(\Theta(t)) =\frac{1}{2}[Q^2(t+1)-Q^2(t) ] 
    &=\frac{1}{2}\Big[\Big(max[Q(t) + E(t) - E_{avg}, 0]\Big)^2-Q^2(t)\Big] \\
    &\le \frac{1}{2}\Big(E_{avg}^{2}+E^{2}_{max} + Q(t)[E(t) - E_{avg}]\Big).
\end{aligned}
\end{equation}
\end{small}
By adding the time cost, we have:
\begin{small}
\begin{equation}
\label{Combining ineq}
\begin{aligned}
    &\Delta(\Theta(t)) + V\sum_{k = 1}^{N}\mathbb{E}\Big[T^k(t)|\Theta(t)\Big]  \le V\sum_{k = 1}^{N}\mathbb{E}\Big[T^k(t)|\Theta(t)\Big]  
    + Q(t)\mathbb{E}\Big[E(t) - E_{avg}|\Theta(t)\Big] + B
\end{aligned}
\end{equation}
\end{small}
Note that B is defined as $\frac{1}{2}(E_{avg}^{2}+E^{2}_{max})$, hence we prove Lemma 1.
\end{IEEEproof}

\section{\textbf{Proof of Theorem1}}  
\label{Nashe}
Before proving the theorem 1, we introduce two lemmas. One (Lemma 3) is associated with the improvement path where each service migrates to the next service migration position; Another (Lemma 4) is associated with the improvement path where each service migrates from the last service migration position. 
\begin{lemma}
	\label{best-response-improvement-path}
	If $j(0), j(1),..., j(R)$ is a sequence of placement decision-making by adopting best response update strategy, $\textbf{c}(0), \textbf{c}(1),..., \textbf{c}(R)$ is the service placement profile for all services at the $r^{th}$ update round ($r = 1, 2, ..., R$), and $\textbf{c}(r)$ results from the migration of a service from $j(r-1)$ to $j(r)$, then $R \le N$, where $N$ is the amount of mobile users and $R$ is the terminal update round.
\end{lemma}
Proof: \textbf{Lemma \ref{best-response-improvement-path}}: Let  $(g_1(r), g_2(r),..., g_M(r))$ be the number of served services in each MEC node under the $r^{th}$ update round. And the minimum amount of served services for each MEC node over the policy update can be denoted as the set $(g_i)_{min} = \min_{r} g_i(r)$ $(1 \le i \le M)$. Obviously, all the served service amount in each MEC node satisfies the following inequality:
\begin{small}
	\begin{equation}
	\label{updateRelation}
	(g_i)_{min} \le g_i(r) \le (g_i)_{min} + 1, i \in \mathcal{M}, 0\le r\le R,
	\end{equation}
\end{small}
where $\mathcal{M}$ is the set of MEC nodes. Only when a service is migrated to MEC node $i$ (i.e., $i = j(r)$), the equality on the right is satisfied; Reversely. when a service is migrated from MEC node $i$ or the state of MEC node $i$ keeps unchanged (i.e., $i \ne j(r)$), the equality on the left is satisfied. Hence migrating the selected service to MEC node $i$ (i.e., $i = j(r)$) at the $r^{th}$ update round will bring $g_i(r)$ to the maximum and all others MEC nodes will achieve the minimum service amount. For the monotonicity of the user QoS objective functions (i.e., the increasing amount of served service will cause the user performance deterioration), $j(r)$ is still a best response for the user in all subsequent update rounds after it is migrated to $j(r)$. Clearly, each service will be migrated at most once.

\begin{lemma}
	\label{b}
	Similarly, if the service migration in the $r^{th}$ round is from $j(r)$ to $j(r-1)$, then $R\le N(M-1)$, where $M$ is the number of MEC nodes.
\end{lemma}
Proof: \textbf{Lemma \ref{b}}: The inequality $(g_i)_{min} \le g_i(r) \le (g_i)_{min} + 1$ also holds for this improvement path. Different from the former, the equality on the left holds when a service is migrated from MEC node $i$ (i.e., $i = j(r)$). Obviously, the service migration in the $r^{th}$ round brings the number of served services in MEC node $j(r)$ to its minimum. This update demonstrates the cost of migrated service in MEC node $j(r)$ is larger than in MEC node $j(r-1)$, due to the definition of the best response update. Therefore, any service will not return to the MEC nodes which it has been ever migrated from. Further, it implies each service is migrated at most $M-1$ times in this improvement path.
\begin{IEEEproof}	
	The proof proceeds by induction on the amount of mobile users $N$ in the system. For only one user in the system ($N = 1$), the proof is trivial. We assume that in $(N-1)$ service placement problem, the terminal updated service placement profile can reach a Nash equilibrium within $M\tbinom{N}{2}$. Then we will prove the theorem still holds for $N$ service placement problem. 
	
	First, we denote $N$ service placement problem as $\Gamma$. And $(N-1)$ service placement problem is derived from $\Gamma$ by restricting the  last service placement, denoted as $\overline{\Gamma}$.

	Based on the induction hypothesis, there exists a service placement profile $\overline{\textbf{c}} = ({c}_1, {c}_2,..., {c}_{N-1})$ reaching a Nash equilibrium in $(N-1)$ service placement problem. Let $(\overline{g}_1(0), \overline{g}_2(0),..., \overline{g}_M(0))$ be the number of served services in each MEC node. For problem $\Gamma$, let ${c}_N(0)$ be a best response for service $N$ against $\overline{\textbf{c}}$. First, the service $N$ will be assigned to the MEC node ${c}_N(0)$. Based on the \textbf{Lemma 3}, we can gain a sequential j(0), j(1), ..., j($R_1$) of placement decisions, where $R_1$ is the maximal update time. If $j(R_1) \neq c_N(0)$, then starting with $\tilde{j}(R_1) = c_N(0)$ against \textbf{c}($R_1$), based on the \textbf{Lemma 4}, we can gain a sequential $\tilde{j}(R_1), \tilde{j}(R_1 + 1), ..., \tilde{j}(R_2)$ placement decisions, where $R_2$ is the maximal update time.	If $j(R_1) = c_N(0)$, then we set $R_1 = R_2$. To both cases, after the $R_2$ times improvement update, we claim the the final placement policy \textbf{c}($R_2$) reach a Nash equilibrium. Suppose the contrary, that $c_k(R_2)$ is not a best response decision for user $k$ against service placement profile $\textbf{c}(R_2)$. Further, we assume the MEC node $j$ is the best response decision for that user. If $c_k(R_2) = c_k(R_2 -1) = ... = c_k(z)$ and $z$ is minimal (i.e., $z = 0$ or $c_k(z) \neq c_k(z-1)$), then based on the improvement path, $c_k(z)$ is the best response update for user $k$ against service placement profile $\textbf{c}(z)$. There are two reasons why the final best response decision is $j$ but not $c_k(R_2)$: (1) $g_{c_k(R_2)}(R_2) > g_{c_k(R_2)}(z)$, (2) $g_j(R_2) < g_j(z)$. According to the improvement path, the reason (2) holds only if $j = \tilde{j}(R_2)$. But it will contradict the maximality of $R_2$, since the service profile of user $k$ will be migrated from $c_k(R_2)$ to $\tilde{j}(R_2)$. The reason (1) holds only if $c_k(R_2) = j(R_1)$ and $k=0$ (i.e., $c_k(0) = c_k(1) = ... = c_k(R_2) = j(R_1)$). By the maximum of $R_1$, $c_k(R_2) = c_k(R_1) = j(R_1)$ must be the best response decision for user $k$ against service placement profile $\textbf{c}(R_1)$. This is because the decision $c_k(R_1) = c_k(0)$ is the best response update for service $k$, which has never been migrated. If $c_k(R_1)$ is not the best response decision, the maximum update times in \textbf{Lemma 3} will be contradicted. Thus $c_k(R_2)$ must be the best response decision for user $k$ against service placement profile $\textbf{c}(R_2)$.
	
	Based on above description, the Nash equilibrium of the n-service placement problem can be derived from the (n-1)-service placement by restricting the $n^th$ service placement decision. Following the induction hypothesis, each improvement update times in current service amount will not be more than MN rounds based on \textbf{Lemma 3 and 4}. Hence, for n-service placement problem, the total best response update times is at most $M\tbinom{N+1}{2}$.

\end{IEEEproof}

\section{\textbf{Proof of Theorem2}}  
 \label{log-sum-station}
\begin{IEEEproof}
	We use the service placement profile \textbf{c} of all user devices to denote the system state of the Markov chain for every user service placement. Because any state can be transited to other state with a certain probability in finite steps, there exits a stationary distribution for the service placement Markov chain.
	If there exists a stationary distribution in our placement policy search, which can be expressed as the following equations:
	\begin{small}
	\begin{eqnarray}
	q_{\textbf{c}}^*(t) q_{\textbf{c},\textbf{c}'}(t) = q_{\textbf{c}'}^*(t) q_{\textbf{c}',\textbf{c}}(t), \forall\textbf{c},\textbf{c}' \in c(t), \forall t \in \mathcal{T}.
	\end{eqnarray}
	To prove it, according to equation (\ref{optimalPolicy}) and (\ref{transfer_prob}), we have the following equation:
	\begin{equation}
	\begin{aligned}
	q_\textbf{c}^*(t)q_{\textbf{c},\textbf{c}'}(t) & = \frac{\alpha \exp(-\frac{1}{2}\beta\Big(U(\textbf{c}',t) - U(\textbf{c},t)\Big)) exp\Big(-\beta U(\textbf{c},t)\Big)}{\sum_{\textbf{c'} \in c(t)}exp\Big(-\beta U(\textbf{c}',t)\Big)} = \frac{\alpha \exp(-\frac{1}{2}\beta\Big(U(\textbf{c}',t) + exp\Big(-\beta U(\textbf{c},t)\Big)}{\sum_{\textbf{c'} \in c(t)}exp\Big(-\beta U(\textbf{c}',t)\Big)}\\
	& = \frac{\alpha \exp(-\frac{1}{2}\beta\Big(U(\textbf{c},t) - U(\textbf{c}',t)\Big)) exp\Big(-\beta U(\textbf{c}',t)\Big)}{\sum_{\textbf{c'} \in c(t)}exp\Big(-\beta U(\textbf{c}',t)\Big)} = q_{\textbf{c}'}^*(t) q_{\textbf{c}',\textbf{c}}(t)
	\end{aligned}
	\end{equation}
	\end{small}
	Hence, we prove the service placement Markov chain is time-reversible, and our algorithm can achieve to a stationary distribution by finite update steps. 
\end{IEEEproof}
\vspace{-20pt}

\section{\textbf{Proof of Theorem 3}}
\label{Long-Sum-Exp}
\begin{IEEEproof}
	\textbf{Long-Sum-Exp Approximation of} $\pmb{\mathcal{P}2}$:
	The minimized objective function value of our system can be approximated by the \textit{long-sum-exp function} over all feasible placement policies as following:
	\begin{small}
	\begin{equation}
	\min_{\textbf{c} \in c(t)} U(\textbf{c},t)  \thickapprox -\frac{1}{\beta}\log\Big[\sum_{\textbf{c} \in c(t)}\exp\Big(-\beta U(\textbf{c},t)\Big)\Big]
	\end{equation}
	\end{small} 
	where $\beta$ is a positive constant that controls the approximation accuracy. Let $|\delta|$ denotes the size of feasible service placement profile of all user devices. Then, we can gain the following inequality:
	\begin{small}
	\begin{equation}
	\label{key}
	0 \le \min_{\textbf{c} \in c(t)}U(\textbf{c},t) + \frac{1}{\beta}\log\Big[\sum_{\textbf{c} \in c(t)}\exp\Big(-\beta U(\textbf{c},t)\Big)\Big]  \le \frac{1}{\beta}\log|\delta|	
	\end{equation} 
	\end{small}
	As stated in \cite{Chen2013}, to achieve close-to-optimal performance, the ratio $\beta$ does not take too large values. According to (\ref{P4}), we construct an approximation optimization problem by adding an entropy term. Based on the accuracy of the long-sum-exp (\ref{key}), we can gain the following inequality: 
	\begin{small}
	\begin{eqnarray}
	0 \le  \overline{S} - S^* \le \frac{1}{\beta}\ln|\delta|
	\end{eqnarray}
	\end{small}
	hence we prove Theorem 3.
\end{IEEEproof}
